# Supplementary material for: Implementing Strassen's Algorithm with BLIS
Source: arXiv:1605.01078 source file (2016-05-03)
Supplement: Supplementary file 1 [file appendix.tex]

%% \section*{Operations for two steps of Strassen}
%% \label{appendix:A}

\begin{figure*}[ht!]
{\footnotesize%
\[
\begin{array}{| l | l |} \hline
\begin{array}{l}
M_{0} = ( A_{0, 0} \!+\! A_{2, 2} \!+\! A_{1, 1} \!+\! A_{3, 3}  )  ( B_{0, 0} +
B_{2, 2} \!+\! B_{1, 1} \!+\! B_{3, 3}  ); \\
 ~~~C_{0, 0} +\!\!= M_{0};
C_{1, 1} +\!\!= M_{0};
C_{2, 2} +\!\!= M_{0};
C_{3, 3} +\!\!= M_{0};
\\
M_{1}  =  ( A_{1, 0} \!+\! A_{3, 2} \!+\! A_{1, 1} \!+\! A_{3, 3}  )  ( B_{0, 0} +
B_{2, 2}  );
\\
  ~~~
C_{1, 0} +\!\!= M_{1};
C_{1, 1} -\!\!= M_{1};
C_{3, 2} +\!\!= M_{1};
C_{3, 3} -\!\!= M_{1}; 
\\
M_{2}  =  ( A_{0, 0} \!+\! A_{2, 2}  )  ( B_{0, 1} \!+\! B_{2, 3} \!+\! B_{1, 1} +
B_{3, 3}  );
\\
  ~~~
C_{0, 1} +\!\!= M_{2};
C_{1, 1} +\!\!= M_{2};
C_{2, 3} +\!\!= M_{2};
C_{3, 3} +\!\!= M_{2};
\\
M_{3}  =  ( A_{1, 1} \!+\! A_{3, 3}  )  ( B_{1, 0} \!+\! B_{3, 2} \!+\! B_{0, 0} +
B_{2, 2}  );
\\
  ~~~
C_{0, 0} +\!\!= M_{3};
C_{1, 0} +\!\!= M_{3};
C_{2, 2} +\!\!= M_{3};
C_{3, 2} +\!\!= M_{3};
\\
M_{4}  =  ( A_{0, 0} \!+\! A_{2, 2} \!+\! A_{0, 1} \!+\! A_{2, 3}  )  ( B_{1, 1} +
B_{3, 3}  );
\\
  ~~~
C_{0, 0} -\!\!= M_{4};
C_{0, 1} +\!\!= M_{4};
C_{2, 2} -\!\!= M_{4};
C_{2, 3} +\!\!= M_{4};
\\
M_{5}  =  ( A_{1, 0} \!+\! A_{3, 2} \!+\! A_{0, 0} \!+\! A_{2, 2}  )  ( B_{0, 0} +
B_{2, 2} \!+\! B_{0, 1} \!+\! B_{2, 3}  );
\\
  ~~~
C_{1, 1} +\!\!= M_{5};
C_{3, 3} +\!\!= M_{5};
\\
M_{6}  =  ( A_{0, 1} \!+\! A_{2, 3} \!+\! A_{1, 1} \!+\! A_{3, 3}  )  ( B_{1, 0} +
B_{3, 2} \!+\! B_{1, 1} \!+\! B_{3, 3}  );
\\
  ~~~
C_{0, 0} +\!\!= M_{6};
C_{2, 2} +\!\!= M_{6};
\\
M_{7}  =  ( A_{2, 0} \!+\! A_{2, 2} \!+\! A_{3, 1} \!+\! A_{3, 3}  )  ( B_{0, 0} +
B_{1, 1}  );
\\
  ~~~
C_{2, 0} +\!\!= M_{7};
C_{3, 1} +\!\!= M_{7};
C_{2, 2} -\!\!= M_{7};
C_{3, 3} -\!\!= M_{7};
\\
M_{8}  =  ( A_{3, 0} \!+\! A_{3, 2} \!+\! A_{3, 1} \!+\! A_{3, 3}  )  ( B_{0, 0}
);
\\
  ~~~
C_{3, 0} +\!\!= M_{8};
C_{3, 1} -\!\!= M_{8};
C_{3, 2} -\!\!= M_{8};
C_{3, 3} +\!\!= M_{8};
\\
M_{9}  =  ( A_{2, 0} \!+\! A_{2, 2}  )  ( B_{0, 1} \!+\! B_{1, 1}  );
\\
  ~~~
C_{2, 1} +\!\!= M_{9};
C_{3, 1} +\!\!= M_{9};
C_{2, 3} -\!\!= M_{9};
C_{3, 3} -\!\!= M_{9};
\\
M_{10}  =  ( A_{3, 1} \!+\! A_{3, 3}  )  ( B_{1, 0} \!+\! B_{0, 0}  );
\\
  ~~~
C_{2, 0} +\!\!= M_{10};
C_{3, 0} +\!\!= M_{10};
C_{2, 2} -\!\!= M_{10};
C_{3, 2} -\!\!= M_{10};
\\
M_{11} = ( A_{2, 0} \!+\! A_{2, 2} \!+\! A_{2, 1} \!+\! A_{2, 3}  )  ( B_{1, 1}
); \\
  ~~~
C_{2, 0} -\!\!= M_{11};
C_{2, 1} +\!\!= M_{11};
C_{2, 2} +\!\!= M_{11};
C_{2, 3} -\!\!= M_{11};
\\
M_{12}  =  ( A_{3, 0} \!+\! A_{3, 2} \!+\! A_{2, 0} \!+\! A_{2, 2}  )  ( B_{0, 0} +
B_{0, 1}  );
\\
  ~~~
C_{3, 1} +\!\!= M_{12};
C_{3, 3} -\!\!= M_{12};
\\
M_{13}  =  ( A_{2, 1} \!+\! A_{2, 3} \!+\! A_{3, 1} \!+\! A_{3, 3}  )  ( B_{1, 0} +
B_{1, 1}  );
\\
  ~~~
C_{2, 0} +\!\!= M_{13};
C_{2, 2} -\!\!= M_{13};
\\
M_{14}  =  ( A_{0, 0} \!+\! A_{1, 1}  )  ( B_{0, 2} \!+\! B_{2, 2} \!+\! B_{1, 3} +
B_{3, 3}  );
\\
  ~~~
C_{0, 2} +\!\!= M_{14};
C_{1, 3} +\!\!= M_{14};
C_{2, 2} +\!\!= M_{14};
C_{3, 3} +\!\!= M_{14};
\\
M_{15}  =  ( A_{1, 0} \!+\! A_{1, 1}  )  ( B_{0, 2} \!+\! B_{2, 2}  );
\\
  ~~~
C_{1, 2} +\!\!= M_{15};
C_{1, 3} -\!\!= M_{15};
C_{3, 2} +\!\!= M_{15};
C_{3, 3} -\!\!= M_{15};
\\
M_{16}  =  ( A_{0, 0}  )  ( B_{0, 3} \!+\! B_{2, 3} \!+\! B_{1, 3} \!+\! B_{3, 3}
);
\\
  ~~~
C_{0, 3} +\!\!= M_{16};
C_{1, 3} +\!\!= M_{16};
C_{2, 3} +\!\!= M_{16};
C_{3, 3} +\!\!= M_{16};
\\
M_{17}  =  ( A_{1, 1}  )  ( B_{1, 2} \!+\! B_{3, 2} \!+\! B_{0, 2} \!+\! B_{2, 2}
);
\\
  ~~~
C_{0, 2} +\!\!= M_{17};
C_{1, 2} +\!\!= M_{17};
C_{2, 2} +\!\!= M_{17};
C_{3, 2} +\!\!= M_{17};
\\
M_{18} = ( A_{0, 0} \!+\! A_{0, 1}  )  ( B_{1, 3} \!+\! B_{3, 3}  ); \\
  ~~~
C_{0, 2} -\!\!= M_{18};
C_{0, 3} +\!\!= M_{18};
C_{2, 2} -\!\!= M_{18};
C_{2, 3} +\!\!= M_{18};
\\
M_{19}  =  ( A_{1, 0} \!+\! A_{0, 0}  )  ( B_{0, 2} \!+\! B_{2, 2} \!+\! B_{0, 3} +
B_{2, 3}  );
\\
  ~~~
C_{1, 3} +\!\!= M_{19};
C_{3, 3} +\!\!= M_{19};
\\
M_{20}  =  ( A_{0, 1} \!+\! A_{1, 1}  )  ( B_{1, 2} \!+\! B_{3, 2} \!+\! B_{1, 3} +
B_{3, 3}  );
\\
  ~~~
C_{0, 2} +\!\!= M_{20};
C_{2, 2} +\!\!= M_{20};
\\
M_{21}  =  ( A_{2, 2} \!+\! A_{3, 3}  )  ( B_{2, 0} \!+\! B_{0, 0} \!+\! B_{3, 1} +
B_{1, 1}  );
\\
  ~~~
C_{0, 0} +\!\!= M_{21};
C_{1, 1} +\!\!= M_{21};
C_{2, 0} +\!\!= M_{21};
C_{3, 1} +\!\!= M_{21};
\\
M_{22}  =  ( A_{3, 2} \!+\! A_{3, 3}  )  ( B_{2, 0} \!+\! B_{0, 0}  );
\\
  ~~~
C_{1, 0} +\!\!= M_{22};
C_{1, 1} -\!\!= M_{22};
C_{3, 0} +\!\!= M_{22};
C_{3, 1} -\!\!= M_{22};
\\
M_{23}  =  ( A_{2, 2}  )  ( B_{2, 1} \!+\! B_{0, 1} \!+\! B_{3, 1} \!+\! B_{1, 1}
);
\\
  ~~~
C_{0, 1} +\!\!= M_{23};
C_{1, 1} +\!\!= M_{23};
C_{2, 1} +\!\!= M_{23};
C_{3, 1} +\!\!= M_{23};
\\
M_{24}  =  ( A_{3, 3}  )  ( B_{3, 0} \!+\! B_{1, 0} \!+\! B_{2, 0} \!+\! B_{0, 0}
);
\\
  ~~~
C_{0, 0} +\!\!= M_{24};
C_{1, 0} +\!\!= M_{24};
C_{2, 0} +\!\!= M_{24};
C_{3, 0} +\!\!= M_{24};
\\
\end{array}
%%% \]
%%% }
%%% {
%%% \footnotesize
%%% \[
&
\begin{array}{@{}l@{}}
M_{25} = ( A_{2, 2} \!+\! A_{2, 3}  )  ( B_{3, 1} \!+\! B_{1, 1}  ); \\
  ~~~
C_{0, 0} -\!\!= M_{25};
C_{0, 1} +\!\!= M_{25};
C_{2, 0} -\!\!= M_{25};
C_{2, 1} +\!\!= M_{25};
\\
M_{26}  =  ( A_{3, 2} \!+\! A_{2, 2}  )  ( B_{2, 0} \!+\! B_{0, 0} \!+\! B_{2, 1} +
B_{0, 1}  );
\\
  ~~~
C_{1, 1} +\!\!= M_{26};
C_{3, 1} +\!\!= M_{26};
\\
M_{27}  =  ( A_{2, 3} \!+\! A_{3, 3}  )  ( B_{3, 0} \!+\! B_{1, 0} \!+\! B_{3, 1} +
B_{1, 1}  );
\\
  ~~~
C_{0, 0} +\!\!= M_{27};
C_{2, 0} +\!\!= M_{27};
\\
M_{28} = ( A_{0, 0} \!+\! A_{0, 2} \!+\! A_{1, 1} \!+\! A_{1, 3}  )  ( B_{2, 2} +
B_{3, 3}  ); \\
  ~~~
C_{0, 0} -\!\!= M_{28};
C_{1, 1} -\!\!= M_{28};
C_{0, 2} +\!\!= M_{28};
C_{1, 3} +\!\!= M_{28};
\\
M_{29} = ( A_{1, 0} \!+\! A_{1, 2} \!+\! A_{1, 1} \!+\! A_{1, 3}  )  ( B_{2, 2}
);\\
  ~~~
C_{1, 0} -\!\!= M_{29};
C_{1, 1} +\!\!= M_{29};
C_{1, 2} +\!\!= M_{29};
C_{1, 3} -\!\!= M_{29};
\\
M_{30} = ( A_{0, 0} \!+\! A_{0, 2}  )  ( B_{2, 3} \!+\! B_{3, 3}  ); \\
  ~~~
C_{0, 1} -\!\!= M_{30};
C_{1, 1} -\!\!= M_{30};
C_{0, 3} +\!\!= M_{30};
C_{1, 3} +\!\!= M_{30};
\\
M_{31} = ( A_{1, 1} \!+\! A_{1, 3}  )  ( B_{3, 2} \!+\! B_{2, 2}  ); \\
  ~~~
C_{0, 0} -\!\!= M_{31};
C_{1, 0} -\!\!= M_{31};
C_{0, 2} +\!\!= M_{31};
C_{1, 2} +\!\!= M_{31};
\\
M_{32}  =  ( A_{0, 0} \!+\! A_{0, 2} \!+\! A_{0, 1} \!+\! A_{0, 3}  )  ( B_{3, 3}
);
\\
  ~~~
C_{0, 0} +\!\!= M_{32};
C_{0, 1} -\!\!= M_{32};
C_{0, 2} -\!\!= M_{32};
C_{0, 3} +\!\!= M_{32};
\\
M_{33} = ( A_{1, 0} \!+\! A_{1, 2} \!+\! A_{0, 0} \!+\! A_{0, 2}  )  ( B_{2, 2} +
B_{2, 3}  );\\
  ~~~
C_{1, 1} -\!\!= M_{33};
C_{1, 3} +\!\!= M_{33};
\\
M_{34} = ( A_{0, 1} \!+\! A_{0, 3} \!+\! A_{1, 1} \!+\! A_{1, 3}  )  ( B_{3, 2} +
B_{3, 3}  ); \\
  ~~~
C_{0, 0} -\!\!= M_{34};
C_{0, 2} +\!\!= M_{34};
\\
M_{35}  =  ( A_{2, 0} \!+\! A_{0, 0} \!+\! A_{3, 1} \!+\! A_{1, 1}  )  ( B_{0, 0} +
B_{0, 2} \!+\! B_{1, 1} \!+\! B_{1, 3}  );
\\
  ~~~
C_{2, 2} +\!\!= M_{35};
C_{3, 3} +\!\!= M_{35};
\\
M_{36}  =  ( A_{3, 0} \!+\! A_{1, 0} \!+\! A_{3, 1} \!+\! A_{1, 1}  )  ( B_{0, 0} +
B_{0, 2}  );
\\
  ~~~
C_{3, 2} +\!\!= M_{36};
C_{3, 3} -\!\!= M_{36};
\\
M_{37}  =  ( A_{2, 0} \!+\! A_{0, 0}  )  ( B_{0, 1} \!+\! B_{0, 3} \!+\! B_{1, 1} +
B_{1, 3}  );
\\
  ~~~
C_{2, 3} +\!\!= M_{37};
C_{3, 3} +\!\!= M_{37};
\\
M_{38}  =  ( A_{3, 1} \!+\! A_{1, 1}  )  ( B_{1, 0} \!+\! B_{1, 2} \!+\! B_{0, 0} +
B_{0, 2}  );
\\
  ~~~
C_{2, 2} +\!\!= M_{38};
C_{3, 2} +\!\!= M_{38};
\\
M_{39} = ( A_{2, 0} \!+\! A_{0, 0} \!+\! A_{2, 1} \!+\! A_{0, 1}  )  ( B_{1, 1} +
B_{1, 3}  ); \\
  ~~~
C_{2, 2} -\!\!= M_{39};
C_{2, 3} +\!\!= M_{39};
\\
M_{40}  =  ( A_{3, 0} \!+\! A_{1, 0} \!+\! A_{2, 0} \!+\! A_{0, 0}  )  ( B_{0, 0} +
B_{0, 2} \!+\! B_{0, 1} \!+\! B_{0, 3}  );
\\
  ~~~
C_{3, 3} +\!\!= M_{40};
\\
M_{41}  =  ( A_{2, 1} \!+\! A_{0, 1} \!+\! A_{3, 1} \!+\! A_{1, 1}  )  ( B_{1, 0} +
B_{1, 2} \!+\! B_{1, 1} \!+\! B_{1, 3}  );
\\
  ~~~
C_{2, 2} +\!\!= M_{41};
\\
M_{42}  =  ( A_{0, 2} \!+\! A_{2, 2} \!+\! A_{1, 3} \!+\! A_{3, 3}  )  ( B_{2, 0} +
B_{2, 2} \!+\! B_{3, 1} \!+\! B_{3, 3}  );
\\
  ~~~
C_{0, 0} +\!\!= M_{42};
C_{1, 1} +\!\!= M_{42};
\\
M_{43}  =  ( A_{1, 2} \!+\! A_{3, 2} \!+\! A_{1, 3} \!+\! A_{3, 3}  )  ( B_{2, 0} +
B_{2, 2}  );
\\
  ~~~
C_{1, 0} +\!\!= M_{43};
C_{1, 1} -\!\!= M_{43};
\\
M_{44}  =  ( A_{0, 2} \!+\! A_{2, 2}  )  ( B_{2, 1} \!+\! B_{2, 3} \!+\! B_{3, 1} +
B_{3, 3}  );
\\
  ~~~
C_{0, 1} +\!\!= M_{44};
C_{1, 1} +\!\!= M_{44};
\\
M_{45}  =  ( A_{1, 3} \!+\! A_{3, 3}  )  ( B_{3, 0} \!+\! B_{3, 2} \!+\! B_{2, 0} +
B_{2, 2}  );
\\
  ~~~
C_{0, 0} +\!\!= M_{45};
C_{1, 0} +\!\!= M_{45};
\\
M_{46} = ( A_{0, 2} \!+\! A_{2, 2} \!+\! A_{0, 3} \!+\! A_{2, 3}  )  ( B_{3, 1} +
B_{3, 3}  ); \\
  ~~~
C_{0, 0} -\!\!= M_{46};
C_{0, 1} +\!\!= M_{46};
\\
M_{47}  =  ( A_{1, 2} \!+\! A_{3, 2} \!+\! A_{0, 2} \!+\! A_{2, 2}  )  ( B_{2, 0} +
B_{2, 2} \!+\! B_{2, 1} \!+\! B_{2, 3}  );
\\
  ~~~
C_{1, 1} +\!\!= M_{47};
\\
M_{48}  =  ( A_{0, 3} \!+\! A_{2, 3} \!+\! A_{1, 3} \!+\! A_{3, 3}  )  ( B_{3, 0} +
B_{3, 2} \!+\! B_{3, 1} \!+\! B_{3, 3}  );
\\
  ~~~
C_{0, 0} +\!\!= M_{48}; \\
~
\\
~
\end{array}
\\
\hline
\end{array}
\]%
}
\caption{Computations for two levels of Strassen.}
\label{fig:2stepB}
\end{figure*}
